# Supplementary material for: Finite-bias Coulomb blockade thermometry
Source: arXiv:2502.15904 source file (2025-02-21)
Supplement: Supplementary file 1 [file Supplemental_Materials.pdf]

# Supplemental Materials for "Finite-bias Coulomb blockade thermometry"

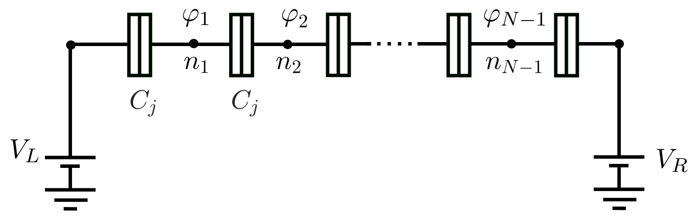


**Fig. S1:** Snapshot of a CBT circuit at a moment between two consecutive tunneling events, where the chain is under a bias voltage $V_L - V_R$ and the $i$-th island has an excess charge $n_i$ and a potential $\varphi_i$. Each junction has a capacitance $C_{\mathrm{j}}$.

# Numerical Methods

## Master Equation

The dynamics of charge transport in an array of $N$ tunnel junctions are described by the master equation, which governs the time evolution of the probability distribution $\sigma(\boldsymbol{n})$ and in the first-order approximation of tunneling can be expressed as [1]

$$\dot{\sigma}(\boldsymbol{n}) = \sum_{\boldsymbol{n'} \in \boldsymbol{n}_{\mathrm{Nbs}}} \left[\sigma(\boldsymbol{n'})\Gamma(\boldsymbol{n'} \to \boldsymbol{n}) - \sigma(\boldsymbol{n})\Gamma(\boldsymbol{n} \to \boldsymbol{n'})\right],$$

where $\boldsymbol{n}$ is a column matrix describing the state of the system, $\boldsymbol{n}^T = (n_1, n_2, \ldots, n_{N-1})$, where each element $n_i$ $(1 < i < N-1)$ represents the number of excess charge on the $i$-th island; see Fig. S1. Here, we take $n_i = 0, \pm1, \pm2, ...$, and define $n_i > 0$ for the number of excess electrons and $n_i < 0$ for excess holes (lack of electrons). The transition rate from state $\boldsymbol{n}$ to $\boldsymbol{n'}$ is denoted as $\Gamma(\boldsymbol{n} \to \boldsymbol{n'})$, and the summation is taken over all the neighboring charge states $\boldsymbol{n}_{\mathrm{Nbs}}$ of state $\boldsymbol{n}$, those states that are accessible states from state $\boldsymbol{n}$ via a single-electron tunneling event. There are $2N$ possible neighboring states for state $\boldsymbol{n}$ which can be shown as columns of the following matrix

$$\mathcal{N} = \begin{pmatrix} n_1{+}1 & n_1{-}1 & n_1 & \cdots & n_1 & n_1{-}1 & n_1{+}1 & \cdots & n_1 \\ n_2 & n_2{+}1 & n_2{-}1 & \cdots & n_2 & n_2 & n_2{-}1 & \cdots & n_2 \\ n_3 & n_3 & n_3{+}1 & \cdots & n_3 & n_3 & n_3 & \cdots & n_3 \\ \vdots & \vdots & \vdots & \ddots & \vdots & \vdots & \vdots & \ddots & \vdots \\ n_{N-1} & n_{N-1} & n_{N-1} & \cdots & n_{N-1}{-}1 & n_{N-1} & n_{N-1} & \cdots & n_{N-1}{+}1 \end{pmatrix}. \tag{S.1}$$

In the steady state, $\dot{\sigma}(\boldsymbol{n}) = 0$, the current passing through the entire chain is the same through each junction. Therefore, once the probability distribution is obtained, one can determine the steady-state current by evaluating the net transition rates over an arbitrary junction. The current thus can be calculated as follows:

$$I = e\sum_{\boldsymbol{n}} \sigma(\boldsymbol{n}) \Big[\Gamma(\boldsymbol{n} \to \{\cdots, n_i-1, n_{i+1}+1, \cdots\}) - \Gamma(\boldsymbol{n} \to \{\cdots, n_i+1, n_{i+1}-1, \cdots\})\Big], \tag{S.2}$$

where $\boldsymbol{n}$ runs over all possible charge states, and $i$ $(i+1)$ refers to the islands before (after) the targeted junction. To clarify, $n_i \pm 1$ and $n_{i+1} \mp 1$ represent the population change of the two adjacent islands, located on either side of the targeted junction, as a single charge is transferred from one to the other. Note that $n_0 \pm 1$ and $n_N \pm 1$ are merely expressing the exchange of a single charge with the source and drain, respectively, in the case where the first or last junction is selected for current computation.

## Tunneling Rates, Free Energy, and Capacitance Matrix

The tunneling rate $\Gamma(\boldsymbol{n} \to \boldsymbol{n'})$ represents the rate at which the system transitions from state $\boldsymbol{n}$ into state $\boldsymbol{n'}$ via tunneling of a single electron and is given by:

$$\Gamma(\boldsymbol{n} \to \boldsymbol{n'}) = \frac{1}{e^2 R_\mathrm{j}} \frac{\Delta G}{\exp\left(\frac{\Delta G}{k_B T_\mathrm{e}}\right) - 1},$$

where $\Delta G = G(\boldsymbol{n'}) - G(\boldsymbol{n})$ is the change in free energy in this transition (tunneling event). The free energy $G$ is defined as [2]:

$$G = \frac{1}{2} C_\mathrm{j} \sum_{i=1}^{N} (\varphi_i - \varphi_{i-1})^2 - V_L Q_L - V_R Q_R, \tag{S.3}$$

with $\varphi_i$ as the potential at $i$-th island, $C_\mathrm{j}$ is the junction capacitance–assumed to be identical for all junctions–and $V_L$, $V_R$ as the applied voltages on the left and right electrodes; see Fig. S1. The charges $Q_L$ and $Q_R$ are:

$$Q_L = C_\mathrm{j}(V_L - \varphi_1) - m_L e, \quad Q_R = C_\mathrm{j}(V_R - \varphi_{N-1}) - m_R e,$$

where $m_L$ ($m_R$) is the number of electrons that have tunneled from the left (right) reservoir through the first (last) junction. The values of $m_L$ and $m_R$ can be negative if the electrons tunnel out of the chain to the reservoirs (holes tunneling in).

To obtain the potentials of the islands $\varphi_i$, we set up a system of equations based on charge conservation. For the $i$-th island, the excess charge $-n_i e$ is related to the potentials of the adjacent islands by

$$-C_{\rm j}\varphi_{i+1} + 2C_{\rm j}\varphi_i - C_{\rm j}\varphi_{i-1} = -n_i e.$$

Note that for the first and last islands one writes

$$-C_{\rm j}\varphi_2 + 2C_{\rm j}\varphi_1 = -n_1 e + C_{\rm j}V_L,$$

and

$$2C_{\rm j}\varphi_{N-1} - C_{\rm j}\varphi_{N-2} = -n_{N-1}e + C_{\rm j}V_R.$$

Here, we exclude the offset charges as we only focus on the universal regime, where the conductance is independent of offset charges. The charge conservation relations can alternatively be expressed in the matrix representation $\mathbf{C}\boldsymbol{\varphi} = \mathbf{Q}_{\boldsymbol{n}}$ as follows

$$\begin{pmatrix} 2C_{\rm j} & -C_{\rm j} & 0 & ... & 0 & 0 \\ -C_{\rm j} & 2C_{\rm j} & -C_{\rm j} & ... & 0 & 0 \\ 0 & -C_{\rm j} & 2C_{\rm j} & ... & 0 & 0 \\ 0 & \ddots & \ddots & \ddots & \vdots & \vdots \\ \vdots & 0 & ... & -C_{\rm j} & 2C_{\rm j} & -C_{\rm j} \\ 0 & 0 & ... & 0 & -C_{\rm j} & 2C_{\rm j} \end{pmatrix} \begin{pmatrix} \varphi_1 \\ \varphi_2 \\ \varphi_3 \\ \vdots \\ \varphi_{N-2} \\ \varphi_{N-1} \end{pmatrix} = \begin{pmatrix} -n_1e+C_{\rm j}V_L \\ -n_2e \\ -n_3e \\ \vdots \\ -n_{N-2}e \\ -n_{N-1}e+C_{\rm j}V_R \end{pmatrix} \tag{S.4}$$

where $\mathbf{C}$ is the capacitance matrix of the system, and $\boldsymbol{\varphi}$ and $\mathbf{Q}_{\boldsymbol{n}}$ are defined as potential and charge matrices of the state $\boldsymbol{n}$, respectively. Note that the matrix relation (S.4) is valid for $N > 2$, while for $N = 2$, one simply obtains

$$\varphi_1 = \frac{-n_1 e + C_{\rm j}V_L + C_{\rm j}V_R}{2C_{\rm j}}. \tag{S.5}$$

Solving $\boldsymbol{\varphi} = \mathbf{C}^{-1}\mathbf{Q}_{\boldsymbol{n}}$ provides the potentials that are needed to calculate $\Delta G(\boldsymbol{n} \to \boldsymbol{n'})$. This energy change can be used to obtain the tunneling rates $\Gamma(\boldsymbol{n} \to \boldsymbol{n'})$ required for the master equation.

## Damped Simple Iteration Method

We employ the Damped Simple Iteration method [3] to iteratively find the steady-state distribution $\sigma(\boldsymbol{n})$. For this, one has to compute the following relation iteratively

$$\sigma_{k+1}(\boldsymbol{n}) = \lambda \frac{\sum\limits_{\boldsymbol{n}' \in \boldsymbol{n}_{\mathrm{Nbs}}} \sigma_k(\boldsymbol{n}')\Gamma(\boldsymbol{n}' \to \boldsymbol{n})}{\sum\limits_{\boldsymbol{n}' \in \boldsymbol{n}_{\mathrm{Nbs}}} \Gamma(\boldsymbol{n} \to \boldsymbol{n}')} + (1-\lambda)\sigma_k(\boldsymbol{n}), \tag{S.6}$$

where $0 < \lambda < 1$ is the damping parameter. In each iteration, the updated distribution $\sigma_{k+1}(\boldsymbol{n})$ is computed based on the previous step's result, $\sigma_k(\boldsymbol{n})$. This process is repeated until convergence is achieved. Arbitrary initial values for the probability distribution $\sigma_0(\boldsymbol{n})$ can be used, but it must satisfy $\sum_{\boldsymbol{n}} \sigma_0(\boldsymbol{n}) = 1$.

## Computation procedure

The computation begins by defining the charge configuration space, which includes all possible charge states the system can take. Since the space is infinite, it is truncated to a maximum allowable charge, $n_{\mathrm{max}}$, per island, ensuring feasibility and accuracy with an appropriately chosen truncation. To clarify, each island is allowed to have an excess charge within the range $-n_{\mathrm{max}} < n_i < n_{\mathrm{max}}$.

At each bias voltage, Eq. S.4 must be solved iteratively to obtain the probability distribution. In this process, each member of the charge configuration space must be visited. For each member, $\sigma_{k+1}(\mathbf{n})$ is computed using the probabilities from the previous step, $\sigma_k(\mathbf{n})$, along with the computed transition rates to/from the neighboring states. The procedure is then repeated for a defined number of iterations until convergence is achieved. In our computations, we found that $\lambda = 0.8$ provided the fastest convergence, and 1500 iterations were used to ensure high accuracy. The current is then computed using Eq. S.2 by summing the contributions of leftward and rightward transitions across a specific junction and visiting all members of the configuration space for which the probability is previously obtained.

To calculate the differential conductance, all the steps above are done for two infinitesimally close bias voltages to obtain $g = \frac{I(V_{\mathrm{b}}+\Delta V_{\mathrm{b}})-I(V_{\mathrm{b}})}{\Delta V_{\mathrm{b}}}$. The voltage incre-

ments, $\Delta V_b$, should be chosen sufficiently small to ensure linearity in taking the derivative. A typical choice is $\Delta V_b = 0.01 \times \Delta V_{\mathrm{FWHM}}$, where

$$\Delta V_{\mathrm{FWHM}} = \frac{5.439 N k_B T_{\mathrm{e}}}{e}$$

represents the known relation for the full width at half maximum (FWHM) of the conductance dip.

We note that this method is practical for short CBT chains but it becomes impractical as the number of junctions increases, because the dimension of the charge configuration space scales as $(2n_{\max} + 1)^{N-1}$.

## Markov Chain Monte Carlo method (MCMC)

We use a somewhat analogous approach and algorithm used in Ref. [4, 5, 6, 7] to perform the MCMC simulation for our CBT system. The algorithm starts by setting up the charge configuration and calculating the initial free energy. This involves establishing the potentials of the islands through the capacitance matrix defined in Eq. S.4. Next, the algorithm proceeds through a predetermined number of steps. During each step, it produces all possible neighboring states, as demonstrated in Eq. S.1. For each neighboring state, the island potentials and free energies are calculated, followed by the computation of transition rates to these states. The winner of the iteration (the fastest event) is determined using a Poisson random generator that provides $2N$ values between 0 and 1, each weighted by the tunneling rates [1]; the event with the shortest duration is chosen as the winner. Accordingly, the initial charge state and free energy are then updated for the next iteration. To calculate the current, we utilize the stochastic sampling method from Ref. [7], which reduces statistical noise in the simulation using a variance reduction method, which effectively spreads the tunneling current over all junctions at each step. Thus, the tunneling time and the transferred charge at iteration $p$ of the MCMC simulations are determined by

$$\Delta t_p = \left( \sum_{i=1}^{N} (\Gamma_i^+ + \Gamma_i^-) \right)^{-1}, \tag{S.7}$$

and

$$\Delta Q_p = e\frac{\sum_i(\Gamma_i^+ - \Gamma_i^-)R_i/R_\Sigma}{\sum_i(\Gamma_i^+ + \Gamma_i^-)}, \tag{S.8}$$

where $\Gamma_i^+$ and $\Gamma_i^-$ denote the transition rates for the two opposing directions across junction $i$. After completing all Monte Carlo iterations, the total current is calculated using $I = \sum_p \Delta Q_p / \sum_p \Delta t_p$. Finally, the differential conductance is obtained similar to the master equation approach as $g = \frac{I(V_\mathrm{b}+\Delta V_\mathrm{b})-I(V_\mathrm{b})}{\Delta V_\mathrm{b}}$.

# Experimental Methods

# Measured Data for Other Samples

The measured data for the Cu1 and Al samples are presented in Fig. S2. Using our method, the conductance traces are converted into temperature traces, similar to Fig. 3 of the main text.

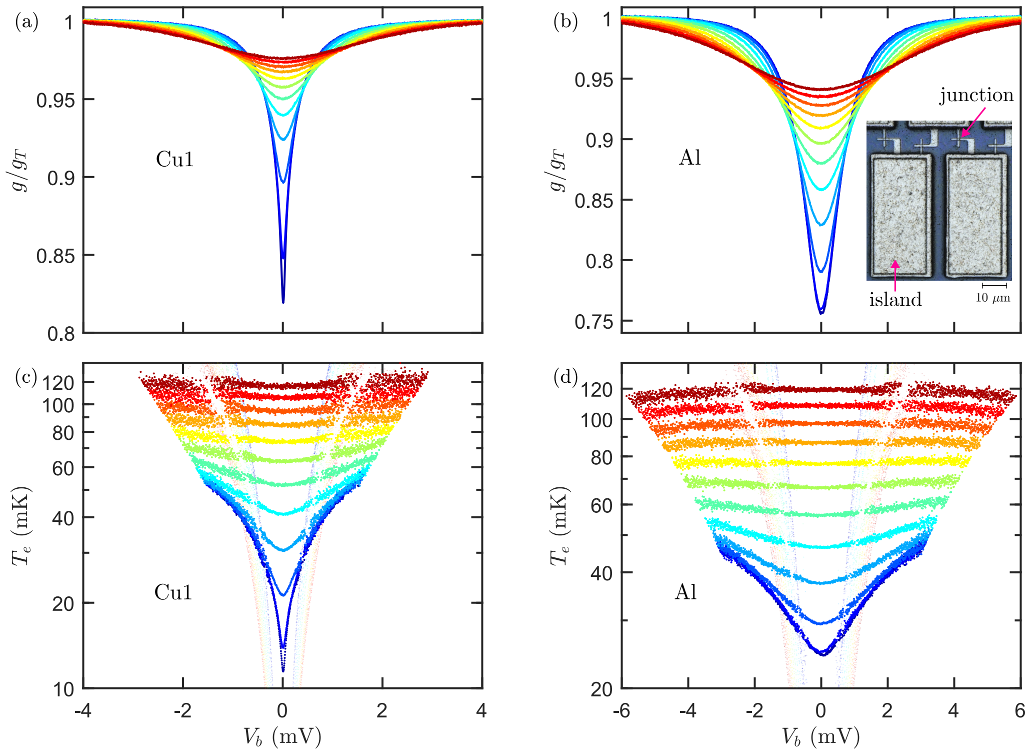


**Fig. S2:** (a) and (b) measured normalized conductance $g/g_\mathrm{T}$ as a function of bias voltage $V_\mathrm{b}$ for Cu1 and Al CBTs, respectively. (c) and (d) Converted conductance traces into temperature traces using our method for the two CBTs, respectively.

## Extraction of $g_{\mathrm{T}}$

As mentioned in the main text, the high bias conductance $g_{\mathrm{T}}$ was obtained via fitting Eq. 1 to the three hottest conductance traces where the heating effects are minimal. The high bias conductance was assumed to be a common fit parameter between the three traces for each sample. The fit results are presented in Fig. S3.

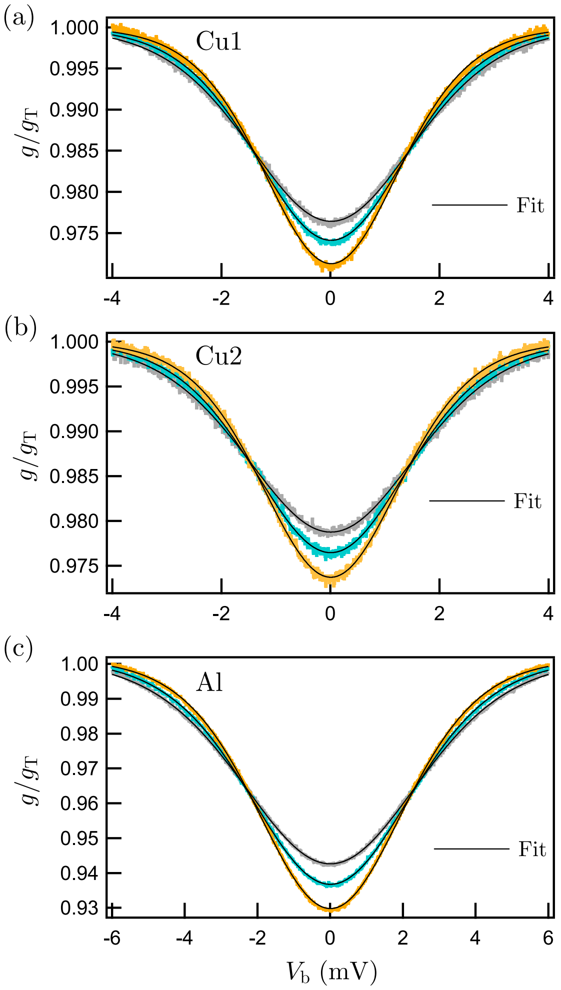


**Fig. S3:** Fit to the three hottest traces yields $g_{\mathrm{T}} = 25.484\ \mu$S for Cu1, $g_{\mathrm{T}} = 21.812\ \mu$S for Cu2, and $g_{\mathrm{T}} = 17.090\ \mu$S for the Al sample, corresponding to junction resistances of $R_{\mathrm{j}} = 4.3$ k$\Omega$, $R_{\mathrm{j}} = 5.0$ k$\Omega$, and $R_{\mathrm{j}} = 5.9$ k$\Omega$, respectively.

## Evolution of Anticrossing vs $E_{\mathrm{c}}$

Here, we demonstrate how the accurate determination of charging energy $E_{\mathrm{c}}$ is crucial for minimizing the anticrossing in temperature traces. Using our conversion method, the conductance trace at $T_{\mathrm{p}} = 35$ mK in Fig. 3(a) is converted into electron

temperature $T_{\mathrm{e}}$. This is repeated for different values of charging energy $E_{\mathrm{c}}$, and the results are presented in Fig. S4 for $E_c/k_B$ ranging between 7.1−7.5 mK. As shown in the left column, the anticrossing appears between the two sets of solutions obtained from the conversion (orange and blue curves). With decreasing charging energy, the anticrossing progressively diminishes and eventually reopens in the opposite direction. This behavior is more clearly illustrated in the zoomed-in views in the middle column. Furthermore, the influence of $E_{\mathrm{c}}$ is evident in the $T_{\mathrm{e}}^5$ versus $V_{\mathrm{b}}^2$ plots, which demonstrate that the data aligns before and after the crossing, at least locally, when the exact charging energy is used for the conversion.

From the above explanation, one can vary the charging energy, track the anticrossing, and identify the exact value of $E_{\mathrm{c}}$ that minimizes the anticrossing. Alternatively, the local linear dependence of $T_{\mathrm{e}}^5$ on $V_{\mathrm{b}}^2$ near the crossing point can be used to minimize the anticrossing for each trace. By fitting two lines to sections of the data—one before and one after $V_{\mathrm{cross}}$—the vertical difference at $V_{\mathrm{cross}}$ is calculated. Then, $E_{\mathrm{c}}$ is iteratively adjusted to minimize this difference. This is how we provided the error bars for the charging energy extraction in the main text, where we repeated this continuity check within ±30% of each $V_{\mathrm{cross}}$ to ensure consistent results.

## Further Demonstration of Dependence of $E_{\mathrm{c}}$ on $T_{\mathrm{p}}$

To further illustrate the dependence of the charging energy on the phonon temperature, we compare the coldest trace and the warmest trace from Fig. 3 and intentionally swap their charging energies. As shown in Fig. S5, using the charging energy from the cold trace on the warm trace (and vice versa) opens the anticrossing and introduces discontinuities in the physical solution. This shows that the charging energy is indeed different for the two traces.

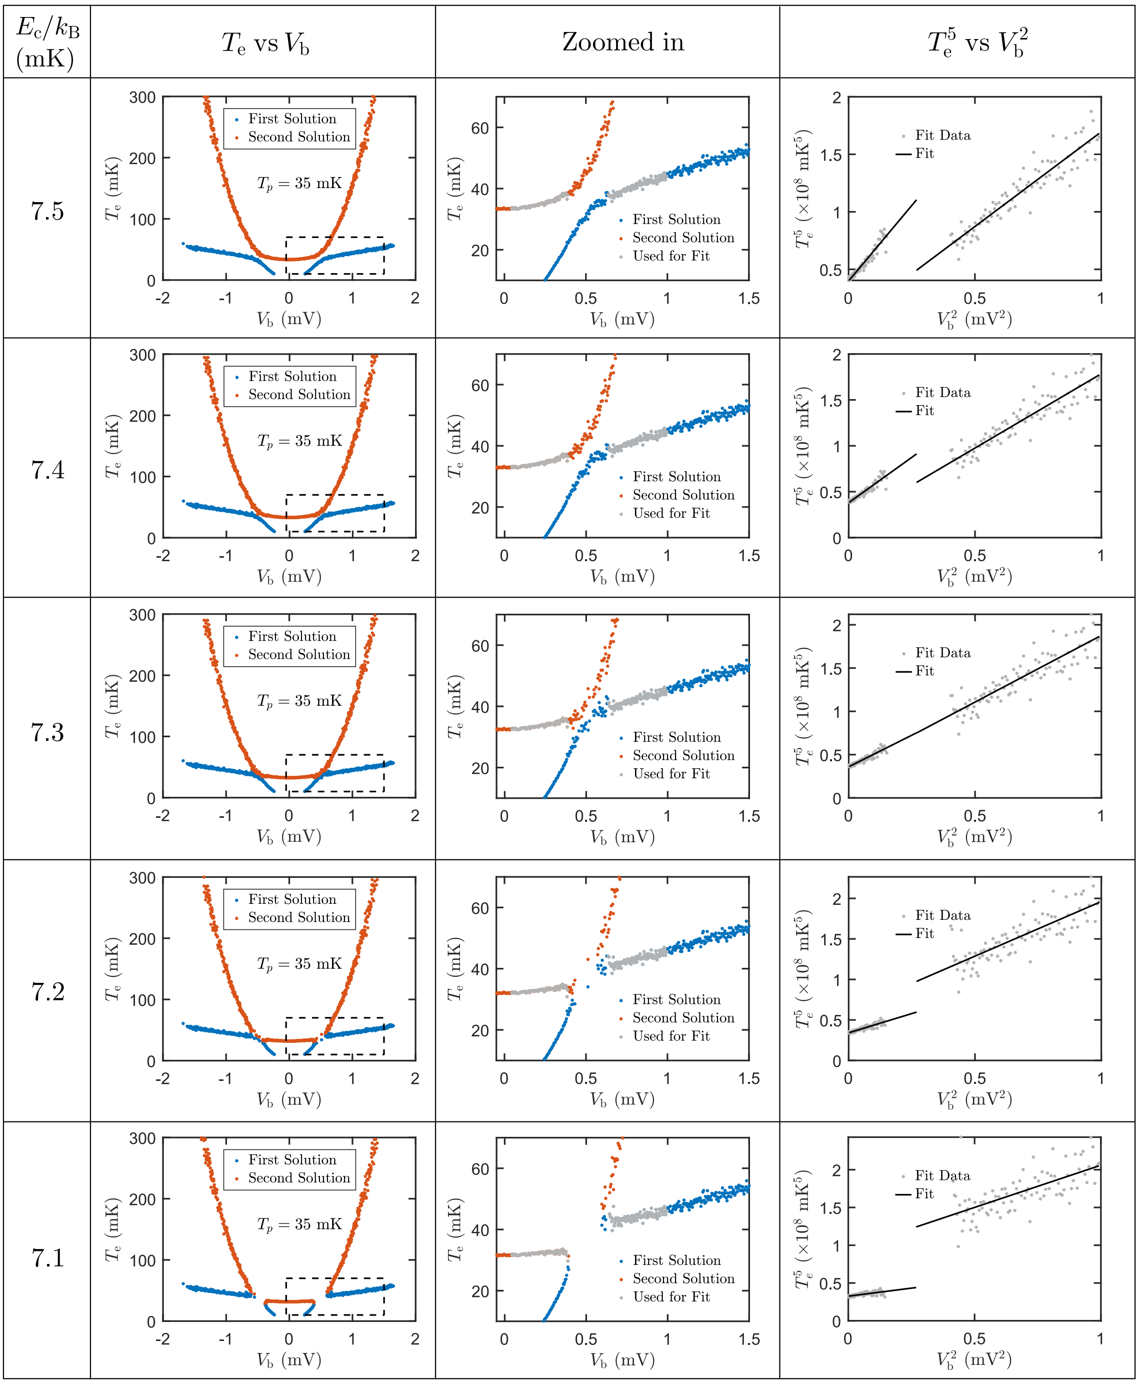


**Fig. S4:** Effect of varying charging energy $E_\mathrm{c}$ on the anticrossing, shown for the conversion of $T_\mathrm{p} = 35$ mK trace in Fig. 3(a). Each row belongs to a specific $E_\mathrm{c}$ value. The first column shows $T_e$ versus $V_b$ with two conversion solutions, the second column provides a zoomed-in view of the anticrossing region, and the third column plots the gray points as $T_e^5$ versus $V_b^2$ along with the linear fits.

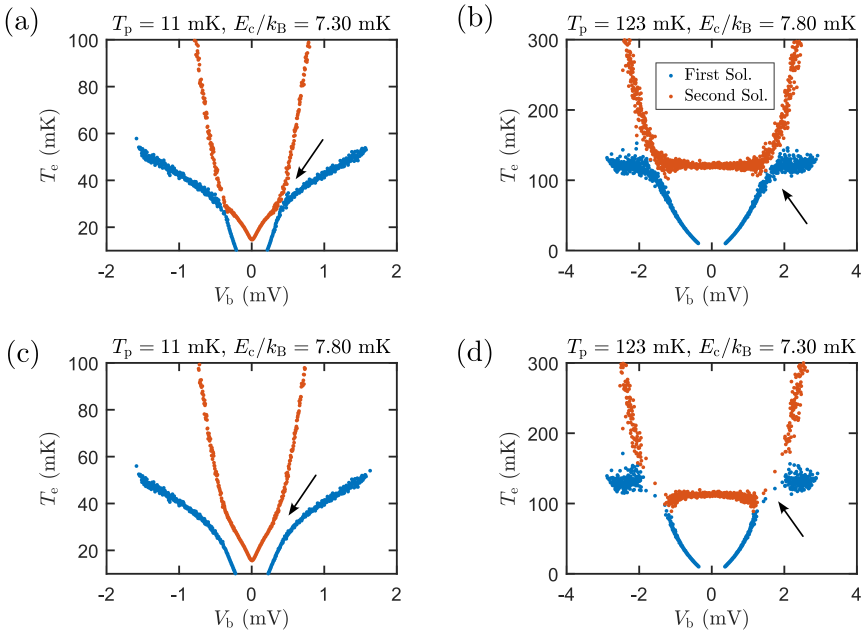


**Fig. S5:** Comparison of $T_\mathrm{p} = 11$ mK and $T_\mathrm{p} = 123$ mK traces for Cu2 sample. (a) and (b) show the traces with their correct charging energies, while (c) and (d) show the effect of swapping the two charging energies.

## Langevin Approach vs. Orthodox Theory

When the resistances of the tunnel junctions are lower than $R_\mathrm{K} = 25.8$ k$\Omega$, the Langevin approach may be used as an alternative to the orthodox theory ($R_\mathrm{j} > R_\mathrm{K}$) to account for higher-order processes. In the universal regime, however, both approaches yield the same results for our samples. For comparison, we also analyzed the data using the Langevin approach from Ref. [8], which produced results in excellent consistency with those obtained using the orthodox theory throughout the paper. The mean dielectric change is plotted in Fig. S7(a) as a function of phonon temperature revealing this consistancy. A slight difference for the Cu1 sample arises from enforcing the same optimization condition in the second method, but this is negligible as both results fall within the same error bar interval (not shown for clarity).

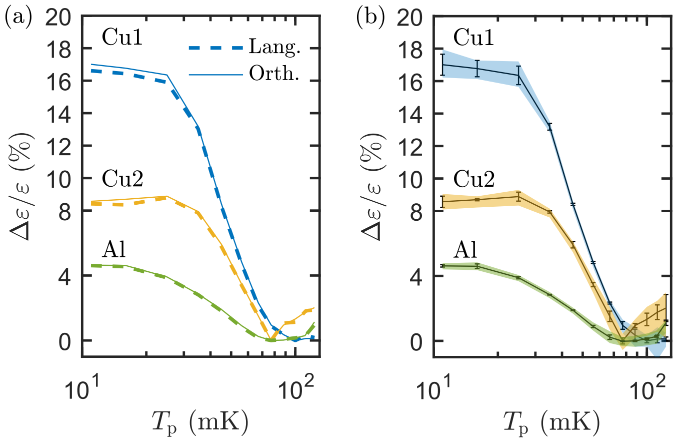


**Fig. S6:** (a) Comparison of the orthodox theory with the Langevin approach for high-conductance tunnel junctions. (b) Effect of constraining $g_\mathrm{T}$ on the results: black curves represent the constrained condition used in the main text, while shaded regions show the errors from the unconstrained condition.

## Effect of Fit Constraint on the Results

As mentioned in the main text, the high bias conductance $g_\mathrm{T}$ was treated as a common fitting parameter in the main text. Removing this constraint introduces negligible uncertainties compared to the constrained, as shown with shaded regions in Fig. S6(b).

## Electron Temperature vs. Dilution Fridge Thermometer

A time trace was recorded at zero bias just before each of the presented bias traces at each $T_\mathrm{p}$. The average CBT conductance of the corresponding time traces is converted into the electron temperature, $T_\mathrm{e}$, using the polynomial relation [9]:

$$1 - \frac{g_0}{g_\mathrm{T}} = \frac{T/T_\mathrm{s}}{6} - \frac{(T/T_\mathrm{s})^2}{60} + \frac{(T/T_\mathrm{s})^3}{630},$$

where $g_0$ and $g_\mathrm{T}$ denote the conductance values at zero bias and high bias, respectively. To perform this conversion, we used the extracted charging energy values corresponding to each phonon temperature; see Fig. 4(c). The resulting $T_\mathrm{e}$ values are plotted against the phonon/refrigerator temperatures, as shown in Fig. S7. This indicates an excellent agreement with the fridge thermometer at high temperatures, while around ~30 mK, the samples Cu1 and Cu2 appear to be colder. This discrep-

ancy may arise from a slight miscalibration of the dilution fridge thermometer, an issue we previously observed with a similar thermometer model elsewhere. We note that for the mentioned data points, the dilution fridge thermometer reads a higher temperature than the actual one. At low temperatures, the sample temperatures tend to saturate due to limitations imposed by weak electron-phonon coupling.

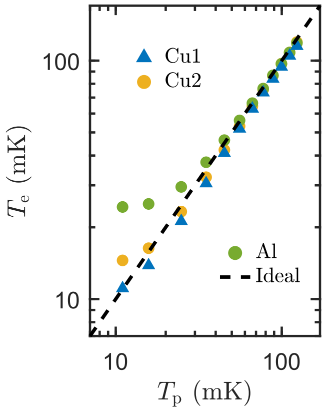


**Fig. S7:** Comparison of electron temperature $T_e$ at zero bias voltage with $T_p$ for the three samples.

# Electron-Phonon Coupling Constant

The power of the phonons for cooling electrons is described by the relationship $P = \Sigma\Omega(T_e^5 - T_p^5)$ in bulk metals [10], where $\Sigma$ is the electron-phonon coupling constant, and $\Omega$ is the volume of the material. By analyzing the dependence of $T_e$ on the dissipated power, as shown in Fig. 4(a), the coupling constant $\Sigma$ can be determined through a linear fit to the data.

For the aluminum sample, this gives $\Sigma = (3.21 \pm 0.02) \times 10^8$ Wm$^{-3}$K$^{-5}$, with the error derived from a linear fit. This value is in agreement with Ref. [11]. However, determining the coupling constant for the copper samples is more complex due to the layered structure, consisting of 150 nm of copper and 60 nm of aluminum on each island. Assuming the contribution of the aluminum layers is negligible, the coupling constants are estimated as $\Sigma = (1.82 \pm 0.06 \pm 0.02) \times 10^9$ Wm$^{-3}$K$^{-5}$ for Cu1 and $\Sigma = (1.9 \pm 0.06 \pm 0.02) \times 10^9$ Wm$^{-3}$K$^{-5}$ for Cu2. The larger error bar originates from the varying area of the islands, while the smaller error bar is taken from the fit.

These values are consistent with those reported in [12]. Thus, the agreement with previously reported values confirms that neglecting the contribution of the aluminum layer is a reasonable assumption, given that aluminum's volume is approximately three times smaller and its coupling constant is about ten times lower than that of copper, with the cooling power depending on the product of these two parameters.

# Bibliography


[1] C. Wasshuber, *Computational Single-Electronics* (Springer Vienna, 2001).

[2] J. A. Melsen, U. Hanke, H.-O. Müller, and K.-A. Chao, Phys. Rev. B **55**, 10638 (1997).

[3] N. Mokhlesi, R. Jazayeri, and D. B. Janes, Superlattice. Microst. **21**, 15 (1997).

[4] N. Bakhvalov, G. Kazacha, K. Likharev, and S. Serdyukova, Sov. Phys. JETP **95**, 1010 (1989).

[5] N. Yurttagül, M. Sarsby, and A. Geresdi, J. Low Temp. Phys. **204**, 143 – 162 (2021).

[6] M. Samani, C. P. Scheller, O. Sharifi Sedeh, D. M. Zumbühl, N. Yurttagül, K. Grigoras, D. Gunnarsson, M. Prunnila, A. T. Jones, J. R. Prance, and R. P. Haley, Phys. Rev. Research **4**, 033225 (2022).

[7] K. P. Hirvi, M. A. Paalanen, and J. P. Pekola, J. Appl. Phys. **80**, 256 (1996).

[8] S. Farhangfar, R. S. Poikolainen, J. P. Pekola, D. S. Golubev, and A. D. Zaikin, Phys. Rev. B **63**, 075309 (2001).

[9] M. Palma, C. P. Scheller, D. Maradan, A. V. Feshchenko, M. Meschke, and D. M. Zumbuhl, Appl. Phys. Lett. **111**, 253105 (2017).

[10] F. C. Wellstood, C. Urbina, and J. Clarke, Phys. Rev. B **49**, 5942 (1994).

[11] M. Meschke, J. Engert, D. Heyer, and J. P. Pekola, Int. J. Thermophys. **32**, 1378 (2011).

[12] M. Meschke, J. P. Pekola, F. Gay, R. E. Rapp, and H. Godfrin, J. Low Temp. Phys. **134**, 1119 (2004).
